# Supplementary material for: Enhancing Mathematical Problem Solving in LLMs through Execution-Driven Reasoning Augmentation
Source: arXiv:2602.03950 source file (2026-02-08)
Supplement: Supplementary file 1 [file efficiency_concerns.tex]

\section{Efficiency Concerns}

While IIPC achieves high accuracy on challenging mathematical benchmarks, we do recognize that it is also a relatively token-intensive approach. While the dual-branch architecture and iterative refinement loop contribute substantially to increased performance as model capacity and problem complexity increase, they also increase prompt length and execution overhead compared to lighter agents such as CoT or PoT. In our implementation of IIPC, the refinement loop allows for 2 process validations and 2 correction runs for each process validation. These values can be directly manipulated according to user needs and tradeoffs. Future work can address this limitation through prompt compression, adaptive refinement depth, direct fine-tuning, and context pruning strategies.
